# Supplementary material for: Stochastic dynamics of granular hopper flows: a configurational mode controls the stability of clogs
Source: arXiv:2312.01194 ancillary file (2025-01-23)
Supplement: Supplementary file 1 [file sm.pdf]

# Supplemental Material for “Stochastic dynamics of granular hopper flows: a configurational mode controls the stability of clogs”

David Hathcock,<sup>1,\*</sup> Sam Dillavou,<sup>2,\*</sup> Jesse M. Hanlan,<sup>2</sup> Douglas J. Durian,<sup>2</sup> and Yuhai Tu<sup>1</sup>

<sup>1</sup>*IBM T. J. Watson Research Center, Yorktown Heights, NY 10598, USA*

<sup>2</sup>*Department of Physics & Astronomy, University of Pennsylvania, Philadelphia, PA 19104, USA*

(Dated: July 9, 2024)

## S1. CLOG STATISTICS IN THE FOUR-STATE MODEL

### A. Distribution of the flow duration with $N$ pauses

As noted in the main text, the total time before clogging, given the trajectory has exactly  $N$  pauses is the sum of  $N + 1$  flow times and  $N$  pause times,

$$T_N = \tau_F^0 + \sum_{i=1}^N \tau_F^i + \tau_P^i, \quad (\text{S1})$$

where  $\tau_F^i$  and  $\tau_P^i$  denote the duration of each flow and pause, which are exponentially distributed with mean  $\tau_{F/P}$ :  $\tau_{F/P}^i \sim \mathcal{E}_{F/P}(t) = \tau_{F/P}^{-1} \exp(-t/\tau_{F/P})$ . The resulting distribution for  $T_N$  is given by a convolution of these exponential distributions,

$$\begin{aligned} p_{T_N}(t) &= \underbrace{\mathcal{E}_F(t) * \mathcal{E}_F(t) * \cdots * \mathcal{E}_F(t)}_{N+1 \text{ times}} * \underbrace{\mathcal{E}_P(t) * \cdots * \mathcal{E}_P(t)}_{N \text{ times}} = \text{Gamma}(N+1, \tau_F) * \text{Gamma}(N, \tau_P) \\ &= \int_0^t \frac{s^N}{N! \tau_F^{N+1}} e^{-s/\tau_F} \cdot \frac{(t-s)^{N-1}}{(N-1)! \tau_P^N} e^{-(t-s)/\tau_P} ds. \end{aligned} \quad (\text{S2})$$

Here  $*$  denotes the convolution, which is written out explicitly in the second line. We use the fact that the sum of  $N$  identically distributed exponential random variables follows a Gamma distribution. Note that the integration limits are finite because the Gamma distribution is zero for negative times. To evaluate the convolution, we separate the integrand into three terms,

$$p_{T_N} = \int_0^t \frac{e^{-t/\tau_F - s/\tau_P}}{N!(N-1)! \tau_F^{N+1} \tau_P^N} \left[ \frac{t}{2} s^{N-1} (t-s)^{N-1} - \frac{1}{2N\mathcal{T}} s^N (t-s)^N + \frac{s^{N-1} (t-s)^{N-1} [N\mathcal{T}(2s-t) + s(t-s)]}{2N\mathcal{T}} \right] ds, \quad (\text{S3})$$

where  $\mathcal{T} = \tau_P \tau_F / (\tau_P - \tau_F)$ . The final term integrates to:  $\exp(-s/\mathcal{T}) s^N (t-s)^N / (2N) \big|_{s=0}^{s=t} = 0$ . The first two terms can be expressed in terms of the modified Bessel function of the first kind  $I_\alpha(x)$ , leading to

$$p_{T_N}(t) = \frac{\sqrt{\pi}}{2N!} \frac{t^{N+1/2} \mathcal{T}^{N-1/2}}{\tau_F^{N+1} \tau_P^N} \exp\left(-\frac{t(\tau_F + \tau_P)}{2\tau_F \tau_P}\right) \left[ I_{N-1/2}\left(\frac{t}{2\mathcal{T}}\right) - I_{N+1/2}\left(\frac{t}{2\mathcal{T}}\right) \right], \quad (\text{S4})$$

The first few distributions are,

$$\begin{aligned} p_{T_0}(t) &= \tau_F^{-1} e^{-t/\tau_F}, \\ p_{T_1}(t) &= \frac{\mathcal{T}^2}{\tau_F^2 \tau_P} e^{-t/\tau_P} - \frac{t\mathcal{T} + \mathcal{T}^2}{\tau_F^2 \tau_P} e^{-t/\tau_F}, \\ p_{T_2}(t) &= \frac{t\mathcal{T}^3 - 3\mathcal{T}^4}{\tau_F^3 \tau_P} e^{-t/\tau_P} + \frac{t^2\mathcal{T}^2 + 4t\mathcal{T}^3 + 6\mathcal{T}^4}{2\tau_F^3 \tau_P^2} e^{-t/\tau_F}. \end{aligned} \quad (\text{S5})$$

This analytical result is compared to the clogging time distributions (conditioned on having  $N$  pauses) in Fig. 2(c) of the main text.

---

\* D.H. and S.D. contributed equally to this work.

### B. Ensemble distribution of the flow duration

The distribution of flow duration across the entire ensemble of flow trajectories is given by  $p_{T_N}(t)$  averaged over the the geometric distribution for the number of pauses  $p(N) = p(1-p)^N$ ,

$$p_T(t) = \sum_{N=0}^{\infty} p_{T_N}(t) p(1-p)^N. \quad (\text{S6})$$

As in the main text,  $p = r_1/(r_0 + r_1)$  is the probability of clogging when the flow rate fluctuates toward zero ( $r_i$  are the switching rates for the hidden variable). This average can be computed in Fourier space. Defining the Fourier transform  $f(\omega) = \mathcal{F}[f(t)] = \int_{-\infty}^{\infty} dt f(t) \exp(i\omega t)$ , the transformed exponential distributions are  $\mathcal{E}_{F/P}(\omega) = 1/(1 - i\omega\tau_{F/P})$ . After Fourier transforming, the convolution in Eq. (S2) becomes a product,

$$\begin{aligned} p_T(\omega) &= \sum_{N=0}^{\infty} \frac{1}{(1 - i\omega\tau_F)^{N+1}} \frac{1}{(1 - i\omega\tau_P)^N} p(1-p)^N \\ &= \frac{p(1 - i\tau_P\omega)}{p - i\omega(\tau_F + \tau_P) - \tau_F\tau_P\omega} \end{aligned} \quad (\text{S7})$$

Taking the inverse Fourier transform leaves us with the distribution quoted in the main text [Eq. (4)],

$$p_T(t) = \frac{c}{\tau_+} e^{-t/\tau_+} + \frac{(1-c)}{\tau_-} e^{-t/\tau_-}, \quad (\text{S8})$$

where  $\tau_{\pm}^{-1}$  are the poles of Eq. (S7)

$$\tau_{\pm} = \frac{2\tau_F\tau_P}{\tau_F + \tau_P \pm \sqrt{(\tau_F + \tau_P)^2 - 4p\tau_F\tau_P}} \quad (\text{S9})$$

and the relative weighting  $c$  is given by,

$$c = \frac{1}{2} + \frac{(2p-1)\tau_P - \tau_F}{2\sqrt{(\tau_F + \tau_P)^2 - 4p\tau_F\tau_P}}. \quad (\text{S10})$$

We find that  $\tau_F$  increases with outlet size  $D$ , while  $\tau_P$  is approximately constant (Fig. S1). As a result, for large outlets we have  $\tau_F \gg \tau_P$ , and the competing time scales become  $c\tau_+ \approx \tau_F/p$  and  $(1-c)\tau_- \approx p(1-p)\tau_P^3/\tau_F^2$ , with the former dominating, resulting in the established exponentially distributed clogging time in this regime [1–5].

### C. Distribution of mass ejected

As mentioned in the main text, because no mass is ejected during the pauses, the total mass ejected over the duration of the entire flow remains exponentially distributed. Following the calculations in the preceding sections, we assume  $m_F$  is the average mass ejected during each flow (preceding a pause or clog). Then the mass ejected in a flow with  $N$  pauses is  $M_N = \sum_{i=0}^N m_F^i$ ; again we assume  $m_F^i$  are exponentially distributed,  $m_F^i \sim \mathcal{E}_M(m) = m_F^{-1} \exp(m/m_F)$ , consistent with Fig. S1(a). It follows that the distribution of mass ejected (given  $N$  pauses) is

$$p_{M_N}(m) = \underbrace{\mathcal{E}_M(m) * \mathcal{E}_M(m) * \dots * \mathcal{E}_M(m)}_{N+1 \text{ times}} = \text{Gamma}(N+1, m_F). \quad (\text{S11})$$

The distribution of mass ejected across all trajectories is (in Fourier space),

$$p_M(\omega) = \sum_{N=0}^{\infty} \frac{1}{(1 - i\omega m_F)^{N+1}} p(1-p)^N = \frac{1}{1 - i\omega m_F/p}, \quad (\text{S12})$$

which corresponds to an exponential distribution with mean  $m_F/p = m_F \langle N+1 \rangle$  (the number of flows is one more than the number of pauses), as quoted in the main text.

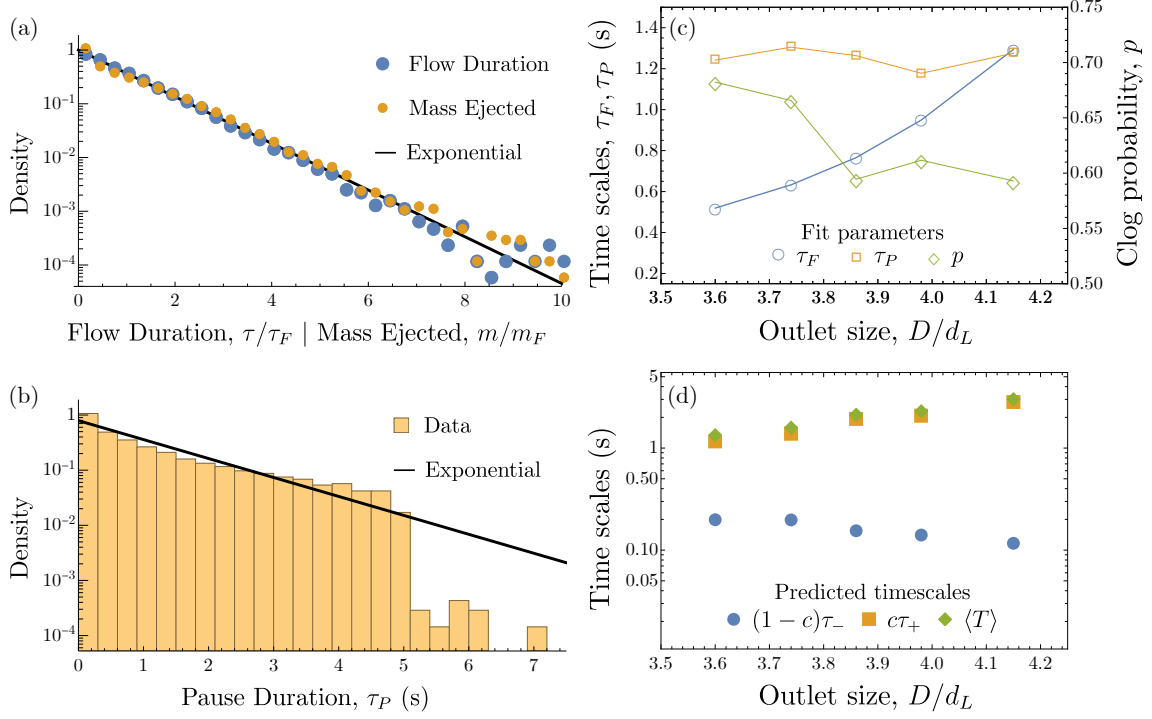

FIG. S1. *Time scales, mass ejected, and outlet-size dependence.* (a) The distributions of flow duration and mass ejected before each pause or clog (normalized by their respective means  $\tau_F = 0.77$  s and  $m_F = 69.4m_L$ ). Each closely follow an exponential distribution. (b) Distribution of pause duration. Note that long pauses ( $\gtrsim 5$  s) are cut off due to the criteria for identifying clogs during automated data collection. The solid line is exponential fit with mean  $\tau_P = 1.26$  s, adjusted to account for the cutoff. Data in (a-b) are from the  $D = 3.86d_L$  dataset. (c) Outlet size dependence of the average flow and pause timescales  $\tau_F$  and  $\tau_P$  and the clog probability  $p$ . (d) Outlet size dependence of the clogging timescales in Eq. (S8) that contribute to the mean  $\langle T \rangle = c\tau_+ + (1-c)\tau_-$ . For larger outlets the single timescale  $c\tau_+$  becomes increasingly dominant.

## S2. ADDITIONAL DATA: FLOW AND PAUSE TIMESCALES, MASS EJECTED, AND OUTLET-SIZE DEPENDENCE

The four-state model calculations in the preceding sections assume that the flow duration and mass ejected preceding a clog or pause as well as the pause duration are each exponentially distributed. Fig. S1(a) shows that the flow duration and mass ejected before each pause or clog do closely follow an exponential distribution (with means  $\tau_F = 0.77$  s and  $m_F = 69.4m_L$  respectively). The pause duration also appears to be exponential [Fig. S1(b)], at least at short times. In this distribution, long-lived pauses  $\gtrsim 5$  s are cutoff because they are classified as permanent clogs during the automated data collection. Previous work on vibrated granular systems suggests the tail of the pause-distribution decays as a power-law [6–9], with exponent decreasing with vibration amplitude. In these studies, however, the power-law scaling is only satisfied for very large and rare pause times that accounting for less than  $1/100^{\text{th}}$  to  $1/10^{\text{th}}$  of pauses depending on experimental conditions. Thus we expect that the exponential approximation will be suitable for capturing statistics of all trajectories except those with very long pauses.

The predictions shown in Fig. 2 of the main text [Eqs. (S4), (S8), and (S12)] also hold across each of the outlet sizes in our dataset  $D/d_L = 3.6, 3.74, 3.86, 3.98$ , and  $4.15$ . Fig. S1(c) shows how the empirical flow and pause timescales  $\tau_F$  and  $\tau_P$  as well as the clog probability  $p$  vary with outlet size. Unsurprisingly, the flow duration  $\tau_F$  increases and the clog probability  $p$  decreases with outlet size. When the outlet is larger, it takes longer to form an arch and these arches are more susceptible to spontaneous declogging. The pause duration  $\tau_P$  is approximately constant with outlet size, though we expect it will decrease if the outlet is large enough; again, arches tend to be less stable when the outlet is larger.

Fig. S1(d) shows the contribution of the two timescales in Eq. (S8), to the mean total clogging time,  $\langle T \rangle = c\tau_+ + (1-c)\tau_-$ . As the outlet size increases, the first time-scale becomes increasingly dominant ( $\langle T \rangle \approx c\tau_+$  and non-exponential features of the clog time diminish). As mentioned in Section S1B, the increase in  $\tau_F$  in Fig. S1(c) implies this behavior: for  $\tau_F \gg \tau_P$  we have  $c\tau_+ \approx \tau_F/p$  and  $(1-c)\tau_- \approx p(1-p)\tau_P^3/\tau_F^2$ , the first of which is dominant.

### S3. FITTING AND ANALYSIS OF THE FOKKER-PLANCK EQUATION

In this section we describe the flow-rate distribution fits and analytical results following from the Fokker-Planck equation for our hidden variable model [Eq. (5) in the main text]. Writing out the dependence on the hidden variable state  $y = 0, 1$  explicitly, the Fokker-Planck equation is given by,

$$\begin{aligned}\frac{\partial P_0}{\partial t} &= -\frac{\partial}{\partial x}(fP_0) + \frac{\partial^2}{\partial x^2}(gP_0) + \frac{x}{x_0}(r_1P_1 - r_0P_0)\theta(x) \\ \frac{\partial P_1}{\partial t} &= -\frac{\partial}{\partial x}(fP_0) + \frac{\partial^2}{\partial x^2}((g + \epsilon)P_0) + \frac{x}{x_0}(r_0P_0 - r_1P_1)\theta(x),\end{aligned}\tag{S13}$$

where  $\theta(x)$  is the Heaviside function. Since there is an absorbing state for  $y = 0$ ,  $P_0(x)$  is defined for  $x > 0$ , while  $P_1(x)$  is defined for all  $x$ . The final term in these equations captures the flow of probability between  $P_0$  and  $P_1$  based on the dynamics of the hidden variable  $y$ . We denote the coupled Fokker-Planck operator by  $\mathcal{L}_{\text{FP}}$ :  $\partial \mathbf{P} / \partial t = \mathcal{L}_{\text{FP}} \mathbf{P}$ , where  $\mathbf{P} = \{P_0, P_1\}$ .

#### A. Deterministic force and flow-rate distribution fitting

The time-dependent flow-rate distributions can be expanded as,  $\mathbf{P}(x, t) = \sum_{i=0}^{\infty} a_i \exp(-\lambda_i t) \mathbf{P}^i(x)$ , in terms of eigenfunctions  $\mathbf{P}^i(x)$  and corresponding eigenvalues  $-\lambda_i$  of the Fokker-Planck operator:  $\mathcal{L}_{\text{FP}} \mathbf{P}^i(x) = -\lambda_i \mathbf{P}^i(x)$ . The constants  $a_i$  are determined by the initial distribution and the eigenvalues are ordered:  $0 < \lambda_0 < \lambda_1 < \dots$ , so that  $\mathbf{P}^0(x)$  is the slowest decaying mode. Assuming a separation of time-scales  $\lambda_0 \ll \lambda_1$ , the distribution of clog times is exponential  $p_T(t) \approx \lambda_0 \exp(-\lambda_0 t)$ , which is consistent with our measurements except at very short times [main text, Fig. 2(d)]. The measured flow-rate distribution is then well approximated by the sum of the components of the slowest decaying mode  $P_0^0(x) + P_1^0(x)$ . All higher-order eigenfunctions quickly decay and the clogging process is dominated by the exponential decay of this single mode.

To compute and fit the leading eigenfunction to measured flow-rate distributions, we discretize the Fokker-Planck operator  $\mathcal{L}_{\text{FP}}$  over a range of  $x$  that is much larger than all measured flow rates. We use the force,

$$f(x) = -\frac{(x - x_0)x^2}{\tau_0 x_0^2} \cdot \frac{x^2 - 2ax + a^2 + b^2}{x_0^2 - 2ax_0 + a^2 + b^2},\tag{S14}$$

which has roots at  $x_0$  and 0 that respectively correspond to the steadily flowing state and the clogged state. The later is taken to be quadratic, so that the clogged state is stable to negative perturbations (flow upward in the hopper), but unstable to positive perturbations (that re-initiate the flow). We also fit forces of the form  $f(x) \propto (x - x_0)(Ax + Bx^2)$ , but the quadratic term was always dominant and including the linear term does not considerably reduce the fitting loss. The second term in Eq. (S14) (denoted  $\Psi(x)$  in the main text) is positive-definite, allowing for deformation of the force without introducing new roots. The factors in the denominator fix the units;  $\tau_0$  is the harmonic decay time near  $x_0$ .

Using Eq. (S14) for the force and linear noise  $g(x) = \Delta x / x_0$ , fitting flow-rate distributions involves tuning 4 parameters  $x_0, a, b, \Delta\tau_0$  (the eigenfunction is independent of the overall time-scale). To fix the scale of  $\Delta$  and  $\tau_0$ , we match the autocorrelation time of the flow rate trajectories to that obtained from simulations, finding  $\tau_0 \approx 20 - 22\text{ms}$  with no clear dependence on  $D$  over this small range of outlet-sizes. We also fix  $p = r_1 / (r_0 + r_1)$  to match the measured geometric pause statistics and choose  $r_0 = (10\tau_0)^{-1}$  so that the switching time-scale for  $y$  is slower than the flow-rate correlation time but faster than the flow and pause times scales. The fit distributions for various outlet sizes are shown in Fig. 3 of the main text.

#### B. Large outlet clogging time and effective noise scaling relation

As shown in Section S2, in the large outlet regime [where  $\tau_F$  grows, see Fig. S1(c)], the average clogging time is  $\langle T \rangle \approx \tau_F / p$ . To compute  $\tau_F$  from the Fokker-Planck equation, we note that the flow duration before a pause or clog does not depend significantly on  $\epsilon \ll 1$ , the noise added by the hidden mode  $y = 1$ . In other words, while the hidden variable state determines the stability of the clog, it has very little impact on the flow preceding a clog or pause. Therefore, we can fix  $y = 0$  and study the one-dimensional Fokker-Planck equation,

$$\frac{\partial P_0}{\partial t} = -\frac{\partial}{\partial x}(fP_0) + \frac{\partial^2}{\partial x^2}(gP_0).\tag{S15}$$

The mean time to hit a clog or pause state ( $x = 0$ ) starting from initial flow rate  $x_i$  satisfies the adjoint equation [10],

$$f(x_i)\tau_F'(x_i) + g(x_i)\tau_F''(x_i) = -1, \quad (\text{S16})$$

with an absorbing boundary at  $x = 0$ ,  $\tau_F(0) = 0$  and reflecting boundary at infinity,  $\lim_{x \rightarrow \infty} \tau_F'(x) = 0$ . The solution to this equation is

$$\tau_F(x_i) = \int_0^{x_i} dy \int_y^\infty dz \frac{e^{\Theta(y) - \Theta(z)}}{g(z)}, \quad (\text{S17})$$

where  $\Theta(x) = -\int_0^x f(x')/g(x') dx'$ . In our flow-rate distribution fits, the steady flow rate  $x_0$  and noise amplitude grow proportionally so that the relative noise  $\tilde{\Delta} = \Delta\tau_0/x_0^2$  shrinks for larger outlet sizes [see inset of Fig. 3(b) in the main text]. Thus when  $D/d_L \gg 1$ , we have  $\tilde{\Delta} \ll 1$ , which appears in the denominator of  $\Theta$ . To approximate the flow duration in this regime, we can therefore evaluate the integrals in Eq. (S17) using a saddle-point approximation. For this analysis we consider deterministic force  $f(x) = -x^2(x - x_0)\Psi(x)/(\tau_0 x_0^2)$  with an arbitrary deformation factor  $\Psi(x)$ . We require  $\Psi(x) > 0$  and  $\Psi(x_0) = 1$  so that the force has no additional roots and the linear correlation time near  $x_0$  is always  $\tau_0$ .

The maximum of the exponent  $\Theta(y) - \Theta(z)$  in Eq. (S17) within the integration domain occurs at  $y_0 = 0$ ,  $z_0 = x_0$ . To quadratic order in  $\delta y = y - y_0$ ,  $\delta z = z - z_0$ , the exponent becomes

$$\Theta(y) - \Theta(z) = -\Theta(x_0) - \frac{\Psi(0)}{2\Delta\tau_0}\delta y^2 - \frac{1}{2\Delta\tau_0}\delta z^2. \quad (\text{S18})$$

Thus, for  $\tilde{\Delta} \ll 1$  the integral in Eq. (S17) reduces to a tightly peaked Gaussian integral around  $(y_0, z_0)$ . Evaluating the integral we find,

$$\langle T \rangle \sim \tau_F/p \sim \frac{2\pi\tau_0 p^{-1}}{\sqrt{\Psi(0)}} e^{-\Theta(x)} = \frac{2\pi\tau_0 p^{-1}}{\sqrt{\Psi(0)}} \exp\left(\frac{1}{\tilde{\Delta}} \int_0^1 \tilde{x}(1 - \tilde{x})\Psi(\tilde{x}x_0)d\tilde{x}\right), \quad (\text{S19})$$

where in the final expression, we have written the exponent explicitly in terms of the effective noise  $\tilde{\Delta}$  and a constant integral. For example, with the force used to fit the experimental flow-rate distributions [Eq. (S14), with  $\Psi(x) = (x^2 - 2ax + a^2 + b^2)/(x_0^2 - 2ax_0 + a^2 + b^2)$ ], we have

$$\langle T \rangle \sim 2\pi\tau_0 p^{-1} \sqrt{1 + \frac{1 - 2\tilde{a}}{\tilde{a}^2 + \tilde{b}^2}} \exp\left(\frac{1}{\tilde{\Delta}} \left[\frac{1}{6} + \frac{1}{60} \frac{10\tilde{a} - 7}{(\tilde{a} - 1)^2 + \tilde{b}^2}\right]\right), \quad (\text{S20})$$

where  $\tilde{a} = a/x_0$  and  $\tilde{b} = b/x_0$ . Suppressing the constants, both Eqs. (S19) and (S20) have the form  $\langle T \rangle \sim \tau_0 p^{-1} C \exp(c\tilde{\Delta}^{-1})$  quoted in the main text.

### C. Clog prediction: first passage to zero flow rate and hidden variable dynamics

Finally, we can use the Fokker-Planck equation to explore whether it is possible to predict clogs given the current flow rate  $x$  and the state of the hidden variable  $y$ . To this end, we compute  $p_0(x)$ , the probability of flow rate hitting zero (either a pause or a clog) before returning to steady flow  $x_0$ , starting from current flow rate  $x$ . We also compute the average time  $t_0(x)$  to hit zero flow (conditioned on this occurring before the system resumes steady flow  $x = x_0$ ), as a measure of how far in advance predictions can be made.

Just as in the preceding section, the flow trajectories before hitting the pause or clog ( $x = 0$ ) or the steady flow state ( $x = x_0$ ) are nearly independent of the hidden variable state  $y$ , since the  $\epsilon$  addition to the noise is only relevant very close to 0. Therefore, we again focus on analyzing the one-dimensional system, Eq. (S15). The zero-flow hitting probability and time satisfy adjoint equations similar to Eq. (S16), but with two absorbing boundaries (i.e. the zero-flow  $x = 0$  and steady flow  $x = x_0$  states) [10],

$$f(x)p_0'(x) + g(x)p_0''(x) = 0 \quad f(x)\vartheta_0'(x) + g(x)\vartheta_0''(x) = -p_0(x). \quad (\text{S21})$$

Here  $\vartheta_0(x) = p_0(x)t_0(x)$  and the boundary conditions are  $p_0(0) = 1$ ,  $p_0(x_0) = 0$ , and  $\vartheta_0(0) = \vartheta_0(x_0) = 0$ . We numerically integrate these equations with force and noise parameters taken from the fits to the experimental flow-rate distributions at each outlet size.

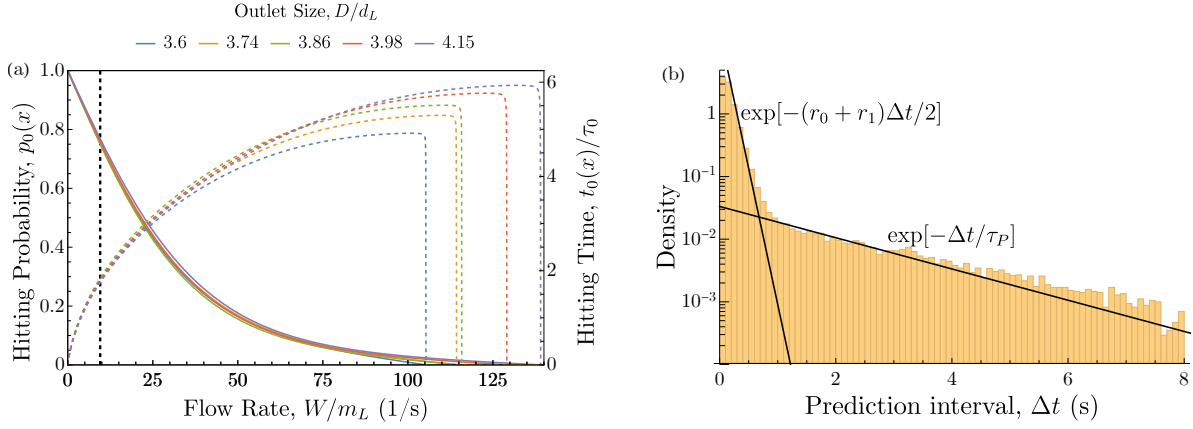

FIG. S2. *Predicting clogs.* (a) The probability  $p_0(x)$  (solid curves) and average time  $t_0(x)$  (dashed curves) for a granular flow with current rate  $x = W/m_L$  to hit zero flow (clog or pause) before returning to steady flow rate  $x_0$ . Curves computed by numerically solving Eq. (S21) with parameters fixed by fitting of the flow-rate distributions (main text, Fig. 3). The black dashed line shows the threshold for 75% probability at  $x \approx 10 \text{ s}^{-1}$ . (b) Distribution of times  $\Delta t$  since the last change in the hidden state  $y$  before a clog or pause. The distribution has two exponential time-scales  $2/(r_0 + r_1)$  and  $\tau_P$ , corresponding respectively to the average  $y$  switching rate and to cases where the flow un-pauses and quickly re-pauses without  $y$  changing state. The  $y$ -state enables distinguishing incipient clogs from pauses  $\langle \Delta t \rangle = 0.27 \text{ s}$  ahead of time on average. Data from  $10^5$  simulated trajectories of the model fit to  $D = 3.86d_L$  trajectories.

Fig. S2(a) shows both the zero-flow hitting probability  $p_0(x)$  and hitting time  $t_0(x)$  for the full range of initial conditions  $0 < x < x_0$ . Accurate prediction of non-flowing events remains difficult due to the Markovian nature for the dynamics. For example, there is only a 75% chance to hit zero flow even when the flow rate is already quite slow ( $x < 10 \text{ s}^{-1}$ ). Fig. S2(a) also shows the average time to hit zero flow is similar to the flow rate correlation time. When the prediction accuracy is 75%, the prediction time is less than  $2\tau_0 \approx 40 \text{ ms}$ .

Clog prediction is further confounded by the presence of pauses: even if the flow ceases, will it restart at a later time? In our model, the hidden variable freezes as the flow rate approaches zero, often well before a pause or clog [e.g. Fig.1(c) in the main text]. Fig. S2(b) shows the distribution of  $\Delta t = t_{x=0} - t_{\delta y}$ , the time interval between the onset of a pause or clog and the previous change in the state of  $y$ ; we find  $\langle \Delta t \rangle = 0.27 \text{ s} \approx 12\tau_0$ . If one could reliably predict zero-flow events, then monitoring the hidden variable state  $y$  would enable advanced determination of whether the incipient clog will be stable or unstable.

#### S4. CONFIGURATIONAL FEATURES OF THE HIDDEN MODE: DISTINGUISHING PAUSE AND CLOG MICROSTATES USING ARCH CONFIGURATIONS AND STATISTICS

To investigate the microscopic configurational features of the hidden mode, we extract pause and clog arches and study various statistics describing the arch shapes. Pauses are isolated in flow trajectories by averaging the instantaneous flow rate over a seven frame ( $\sim 0.05 \text{ s}$ ) moving window. The start and end of a pause are identified by the averaged flow-rate trajectory crossing a threshold  $3 \text{ s}^{-1}$  ( $\sim 3\%$  of the steady flow rate  $x_0$ ). Results are robust to reasonable variations in the averaging window and threshold. For pauses we analyze the frame midway through the duration of the pause, while for clogs we use the final recorded frame. To detect arches from these snapshots, we first compute a Delaunay triangulation of the grain centers and remove links with center-to-center distance larger than 120% of the large grain diameter. Cornerstones of the arch are identified as the grains closest to the corners of the outlet. The arch is then detected by computing the shortest distance path (on the triangulated lattice) between these two grains.

Isolated arches are used to compute the statistics shown in Fig. 4 in the main text. The positional densities are computed by averaging images of the arches across the clog and pause populations. Fig. 4(b) in the main text shows the difference in these densities. The arch statistics are defined as follows: (1) Height,  $h$ : the distance from the hopper floor to the center of the grain with largest vertical position. (2) Width,  $w$ : the maximum horizontal distance between two grain centers in the arch. (3) Angles,  $\theta$ : the signed angle between vectors connecting consecutive grain centers [see Fig.4(a)]. Negative angles correspond to inverted “defect” grains with convex orientation opposing the typical arch curvature. For each arch we compute the minimum angle (the largest defect) and the standard deviation of the angles. The former quantifies the most likely failure mode for the arch, while the later quantifies the irregularity in

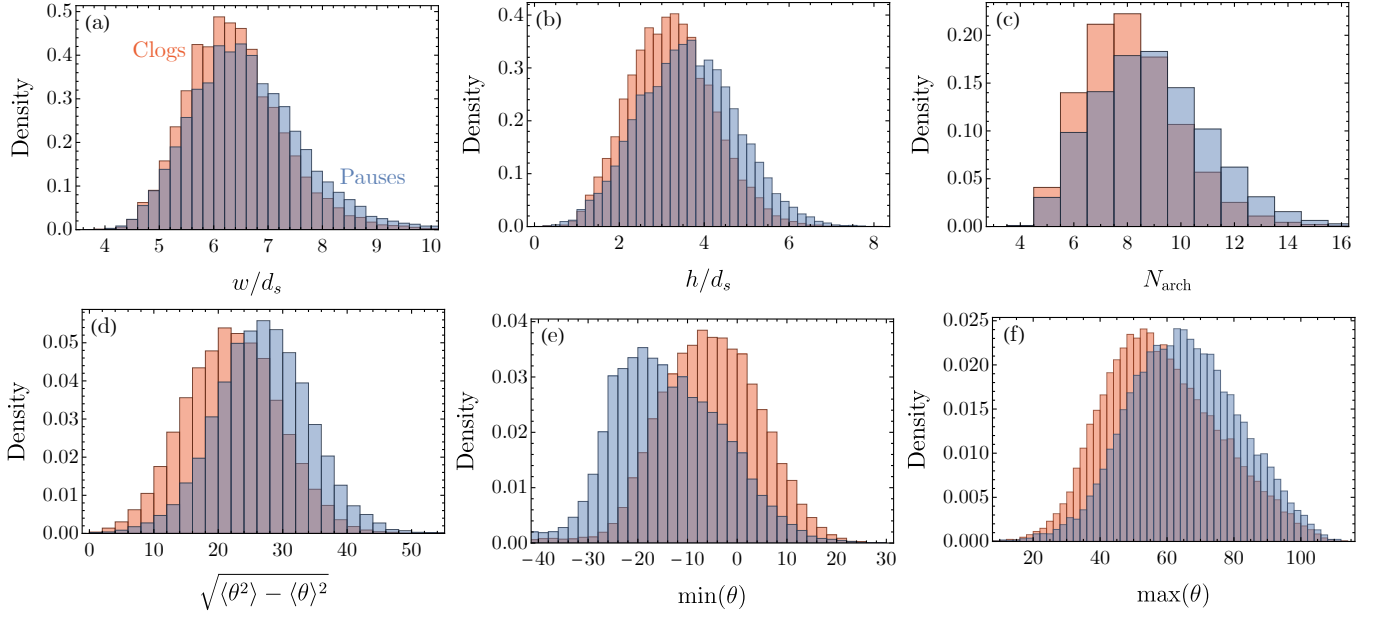

FIG. S3. Distributions of arch statistics for pauses (blue) and clogs (orange). (a) Arch width,  $w$ , (b) Arch height,  $h$ , (c) Number of arch grains,  $N_{\text{arch}}$ , (d) Standard deviation of arch angles,  $\sqrt{\langle\theta^2\rangle - \langle\theta\rangle^2}$ , (e) Minimum arch angle,  $\min(\theta)$ , and (f) Maximum arch angle,  $\max(\theta)$ . Distribution means for (a), (b), (d), and (e) are shown in main text Fig. 4(c) and (d). For pause arches the distributions for each statistic are nearly identical if binned based on pause duration.

arch shape. In addition to these statistics, which were discussed in the main text, we also computed the number of grains in each arch  $N_{\text{arch}}$  and the maximum arch angle.

Fig S3 shows distributions for each of these statistics for the clog and pause arches. While there is a large variation in arch statistics within each population the means are distinctly separated as demonstrated in the main text, Fig. 4(c) and (d); due to our large sample size, the standard error in these means is very small. Individual statistics do not fully separate the two populations, but we conjecture that applying machine learning algorithms [11] to the full positional data could produce a highly accurate classification of pausing versus clogging microstates.

- 
- [1] I. Zuriguel, A. Garcimartín, D. Maza, L. Pagnaloni, and J. Pastor, [Physical Review E](#) **71**, 051303 (2005).
  - [2] K. To, [Phys. Rev. E](#) **71**, 060301 (2005).
  - [3] A. Janda, I. Zuriguel, A. Garcimartín, L. A. Pagnaloni, and D. Maza, [EPL \(Europhysics Letters\)](#) **84**, 44002 (2008).
  - [4] I. Zuriguel, A. Janda, A. Garcimartín, C. Lozano, R. Arévalo, and D. Maza, [Physical Review Letters](#) **107**, 278001 (2011).
  - [5] C. C. Thomas and D. J. Durian, [Physical Review E](#) **87**, 052201 (2013).
  - [6] I. Zuriguel, D. R. Parisi, R. C. Hidalgo, C. Lozano, A. Janda, P. A. Gago, J. P. Peralta, L. M. Ferrer, L. A. Pagnaloni, E. Clément, D. Maza, I. Pagonabarraga, and A. Garcimartín, [Scientific reports](#) **4**, 7324 (2014).
  - [7] C. Merrigan, S. K. Birwa, S. Tewari, and B. Chakraborty, [Phys. Rev. E](#) **97**, 040901 (2018).
  - [8] R. Caitano, B. V. Guerrero, R. E. R. González, I. Zuriguel, and A. Garcimartín, [Phys. Rev. Lett.](#) **127**, 148002 (2021).
  - [9] B. V. Guerrero, B. Chakraborty, I. Zuriguel, and A. Garcimartín, [Phys. Rev. E](#) **100**, 032901 (2019).
  - [10] N. G. van Kampen, *Stochastic processes in physics and chemistry* (Elsevier, Amsterdam, 2007).
  - [11] J. M. Hanlan, S. Dillavou, A. J. Liu, and D. J. Durian, [arXiv preprint arXiv:2407.05491](#) (2024).
